# Supplementary material for: Chaos and correlated avalanches in excitatory neural networks with synaptic plasticity
Source: arXiv:1610.00252 source file (2017-03-17)
Supplement: Supplementary file 1 [file supplemental_arxiv_v2.pdf]

# Chaos and correlated avalanches in neural networks with synaptic plasticity
# (Supplemental material)

Fabrizio Pittorino,[1,2] Miguel Ibáñez-Berganza,[2] Matteo di Volo,[3] Alessandro Vezzani,[4,1,*] and Raffaella Burioni[1,2]

[1]*Dipartimento di Scienze Matematiche, Fisiche e Informatiche, Università di Parma, via G.P. Usberti, 7/A - 43124, Parma, Italy*

[2]*INFN, Gruppo Collegato di Parma, via G.P. Usberti, 7/A - 43124, Parma, Italy*

[3]*Group for Neural Theory, Laboratoire de Neurosciences Cognitives, INSERM U960, Ecole Normale Superieure, Paris, France*

[4]*IMEM-CNR, Parco Area delle Scienze, 37/A-43124 Parma, Italy*

## CONTENTS


I. The Leaky integrate-and-fire (LIF) model with TUM synaptic plasticity 2

II. Mean Field 5

A. Competition of time scales in the Mean Field model 5

B. Weak coupling 6

C. Strong coupling 7

D. Chaos in the Mean Field model 7

E. The limit $\tau_{in} \to 0$ 9

III. Degree based Mean Field 13

A. Event driven dynamics simulation protocol 13

B. Global Synaptic field 14

C. Fluctuations of the interspike interval, Kuramoto parameter and global field 15

D. Lyapunov exponents 17

E. Comparison between the DMF and MF models phase diagrams 18

F. Robustness with respect to the shape of the distribution $P(k_i)$ 19

G. Robustness with respect to the single neuron time scale 20

H. Degree based Mean Field and finite connectivity systems 21

I. Temporal correlations 22

J. Kolmogorov Complexity 24

K. Avalanche size distribution 24

References 25


## I. THE LEAKY INTEGRATE-AND-FIRE (LIF) MODEL WITH TUM SYNAPTIC PLASTICITY

Let us consider a system of $N$ neurons and call $k_i$ the coupling of neuron $i$, where $k_i$ is extracted from the distribution $P(k_i)$[1]. The $Nk_i$ can also be considered as the in-degree of neuron $i$, so that $P(k_i)$ is a degree distribution. The equations of motion of the Degree based Mean Field (DMF)

TUM model are:

$$\begin{aligned}
\dot{v}_i(t) &= a - v_i(t) + gk_i \frac{1}{N}\sum_{j=1}^{N} y_j(t) \\
\dot{y}_i(t) &= -\frac{y_i(t)}{\tau_{in}} + u(1 - y_i(t) - z_i(t))S_i(t) \\
\dot{z}_i(t) &= \frac{y_i(t)}{\tau_{in}} - \frac{z_i(t)}{\tau_R}
\end{aligned} \tag{1}$$

where $v_i(t)$ is reset to 0 at the firing events $t_i(m)$ that correspond to $v_i(t_i(m)) = 1$, and $S_i(t) = \sum_m \delta(t - t_i(m))$ is the spike train of neuron $i$.

Eq.s (1) can be solved by an event driven map[2]. We denote with $v_{i,n}$, $y_{i,n}$ and $z_{i,n}$ the value of $v_i(t_n)$, $y_i(t_n)$ and $z_i(t_n)$ *immediately before the n-th firing event* and with $\Delta_n = t_{n+1} - t_n$ the time interval between the firing events ($t_i(m)$ denotes firing times of neuron $i$ while $t_n$ represents the sequence of firing times of the network, independently of the firing neuron). The evolution of the discrete variables then reads:

$$\begin{aligned}
v_{i,n+1} &= v_{i,n}e^{-\Delta_n} + a(1 - e^{-\Delta_n}) + \frac{gk_i\tau_{\rm in}}{\tau_{\rm in} - 1}\left(e^{-\Delta_n/\tau_{\rm in}} - e^{-\Delta_n}\right)\frac{1}{N}\sum_{j=1}^{N} y_{j,n} \\
y_{i,n+1} &= (y_{i,n} + \delta_{i,s_{n+1}}u(1 - y_{i,n} - z_{i,n}))e^{-\Delta_n/\tau_{\rm in}} \\
z_{i,n+1} &= z_{i,n}e^{-\Delta_n/\tau_{\rm R}} + \frac{\tau_{\rm R}}{\tau_{\rm R} - \tau_{\rm in}}(y_{i,n} + \delta_{i,s_{n+1}}u(1 - y_{i,n} - z_{i,n}))\left(e^{-\Delta_n/\tau_{\rm R}} - e^{-\Delta_n/\tau_{\rm in}}\right),
\end{aligned} \tag{2}$$

where $\delta_{i,j}$ is the Kronecker delta and $s_n$ is the neuron that fires at time $t_n$. To implement the reset rule on the potential, for neuron $s_{n+1}$ that fires at $t_{n+1}$ the first Eq. (2) is replaced by:

$$1 = v_{s_{n+1},n}e^{-\Delta_n} + a(1 - e^{-\Delta_n}) + gk_i\tau_{\rm in}\frac{e^{-\Delta_n/\tau_{\rm in}} - e^{-\Delta_n}}{\tau_{\rm in} - 1}\frac{1}{N}\sum_{j=1}^{N}(y_{j,n} + \delta_{j,s_n}u(1 - y_{j,n} - z_{j,n})) \tag{3}$$

and $v_{s_{n+1},n+1} = 0$. Notice that Eq. (3) allows to calculate $\Delta_n$ and that the firing neuron is identified by finding the value of $s_{n+1}$ that provides the minimum value of $\Delta_n$ in Eq. (3).

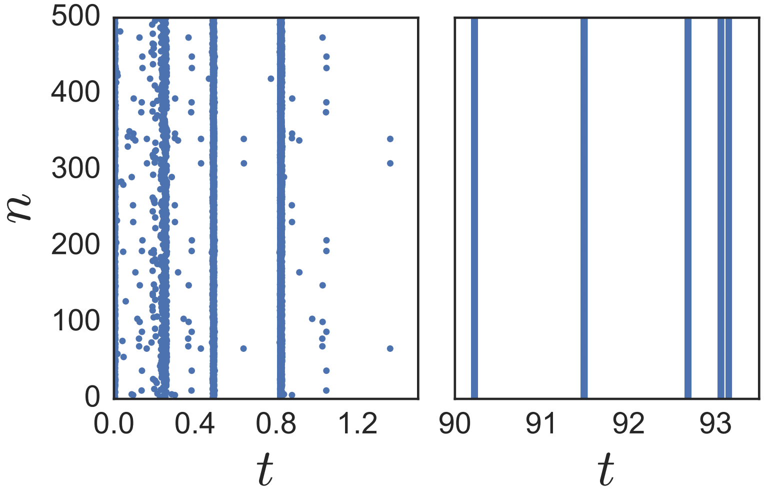


FIG. 1. Raster plot of a fully MF system with $k_i = k_0 = 0.7$, $g = 10^6$ $\tau_{in} = 10^{-3}$ each dot represents the firing event of neuron $n$. Left: short time evolution. Right: in the long time evolution the system reaches a synchronous but chaotic state.

Let us consider the Mean Field (MF) case where $k_i = k_0$ for all sites. In Fig. 1 we report a raster plot showing that the system converges, after a short transient, to a synchronous state where all neurons fire simultaneously. This had already been observed in a parameter setup showing periodic synchronous dynamics[3]. Nevertheless, in the present case the synchronous solution shows an irregular chaotic dynamics, indicating our system as an example of synchronous chaos[4,5]. Since each neuron displays the same dynamical evolution, the MF equations reduce to the dynamics of a single neuron representing the entire system. We can consequently drop the index $i$ and obtain:

$$\begin{aligned}\dot{v}(t) &= a - v(t) + gk_0 y(t)\\ \dot{y}(t) &= -\frac{y(t)}{\tau_{in}} + u(1 - y(t) - z(t))S(t)\\ \dot{z}(t) &= \frac{y(t)}{\tau_{in}} - \frac{z_i(t)}{\tau_R}.\end{aligned} \tag{4}$$

The corresponding event driven map reads

$$\begin{aligned}1 &= a(1 - e^{-\Delta_n}) + \frac{gk_0\tau_{\rm in}}{\tau_{\rm in} - 1}\left(e^{-\Delta_n/\tau_{\rm in}} - e^{-\Delta_n}\right)(y_n + u(1 - y_n - z_n))\\ y_{n+1} &= (y_n + u(1 - y_n - z_n))e^{-\Delta_n/\tau_{\rm in}}\\ z_{n+1} &= z_n e^{-\Delta_n/\tau_R} + \frac{\tau_{\rm R}}{\tau_{\rm R} - \tau_{\rm in}}(y_n + u(1 - y_n - z_n))\left(e^{-\Delta_n/\tau_{\rm R}} - e^{-\Delta_n/\tau_{\rm in}}\right),\end{aligned} \tag{5}$$

where we take into account that the single neuron fires at each event, and therefore we use Eq. (3) with $v_n = 0$. In practice, the first of Eq.s (5) is used to obtain the firing time intervals $\Delta_n$ while the other two equations represent a discrete two dimensional map for the variables $y_n$ and $z_n$.

## II. MEAN FIELD

### A. Competition of time scales in the Mean Field model

The single neuron MF Eq.s (4,5) become particularly simple in the weak coupling and strong coupling regimes. In the former, we can neglect $gk_0y(t)$ in Eq.s (4) while in the latter we neglect $a-v(t)$. In both limits, the map (5) has a fixed point, characterized by a slow and a fast periodicity respectively.

Let us first discuss some general property of the fixed point. We consider the regime $T = \ln(a/(a-1)) \sim O(1)$ and $\tau_{in} \ll T \ll \tau_R$, so that the event driven dynamics (5) of the MF model becomes:

$$1 = a - g\tau_{in}k_0 y_{n+1} - e^{-\Delta_n}\left(a - g\tau_{in}k_0(y_n + u(1-y_n-z_n))\right) \tag{6}$$

$$y_{n+1} = e^{-\frac{\Delta_n}{\tau_{in}}}(y_n + u(1-y_n-z_n)) \tag{7}$$

$$z_{n+1} = -y_{n+1} + e^{-\frac{\Delta_n}{\tau_R}}\left(y_n + z_n + u(1-y_n-z_n)\right). \tag{8}$$

We denote with $(x^*, y^*)$ the fixed point of the map (6-8) and with $\Delta^*$ the relevant interspike interval, i.e. Eq.s (6-8) are satisfied by $y_{n+1} = y_n = y^*$, $x_{n+1} = x_n = x^*$ and $\Delta_{n+1} = \Delta_n = \Delta^*$.

Eq.s (7-8) hold both in the strong and in the weak coupling regimes and they describe a general property of the fixed point. In particular, considering the variable $w^* = y^* + z^*$, Eq. (8) reads:

$$w^* = e^{-\frac{\Delta^*}{\tau_R}}(w^* + u(1-w^*)) \tag{9}$$

and:

$$w^* = u\frac{e^{-\frac{\Delta^*}{\tau_R}}}{1-(1-u)e^{-\frac{t^*}{\tau_R}}} \simeq 1 - \frac{\Delta^*}{u\tau_R}, \tag{10}$$

where in the last step we used our assumption $\Delta^* \ll \tau_R$. Inserting Eq. (10) in Eq. (7), the equation for the fixed point of $y^*$ reads:

$$y^* = e^{-\frac{\Delta^*}{\tau_{in}}}\frac{\Delta^*}{\tau_R}\frac{1}{1-e^{-\frac{\Delta^*}{\tau_{in}}}}. \tag{11}$$

Let us come back to the differential Eq.s (4) and consider the periodic solution corresponding to the fixed point of the map. Since $y^*$ represent the value of $y(t)$ immediately before a firing event, if we set the time axes so that the firing events occur at $t = 0, \Delta^*, 2\Delta^*...$, for $0 < t < \Delta^*$ we have that:

$$y(t) = \frac{\Delta^*}{\tau_R}\frac{e^{-\frac{t}{\tau_{in}}}}{1-e^{-\frac{\Delta^*}{\tau_{in}}}}. \tag{12}$$

We remark that, at the fixed point, the above dynamical evolution holds for any value of the coupling constant. However, the value of $\Delta^*$ is determined by Eq. (6) which explicitly depends on $g$. In particular, in the strong coupling regime Eq. (6) reduces to:

$$1 = -g\tau_{in}k_0 y_{n+1} + g\tau_{in}k_0(y_n + u(1 - y_n - z_n)). \tag{13}$$

Imposing $y^* = y_{n+1} = y_n$ and $z^* = z_{n+1} = z_n$ we get $1 = g\tau_{in}k_0 u(1 - y^* - z^*)$, which gives

$$w^* = 1 - \frac{1}{uk_0 g\tau_{in}}. \tag{14}$$

Comparing Eq. (10) with Eq. (14) we get:

$$\Delta^* = \Delta^*_S \simeq \frac{\tau_R}{g\tau_{in}k_0}. \tag{15}$$

On the other hand, in the weak coupling regime, we obviously obtain $\Delta^* = \Delta^*_W = \ln(\frac{a}{a-1}) \simeq O(1)$.

We now plug (12) into the first of Eq.s (4), describing the evolution of the membrane potentials, and we verify under which conditions the periodicity of the weak and strong coupling regime remains unperturbed. In particular, for $0 < t < \Delta^*$, we have that $v(t)$ satisfies the equation:

$$\dot{v}(t) = a - v(t) + \frac{gk_0\Delta^*}{\tau_R}\frac{e^{-\frac{t}{\tau_{in}}}}{1 - e^{-\frac{\Delta^*}{\tau_{in}}}}. \tag{16}$$

Solving the differential equation and imposing $\tau_{in} \ll 1$, we get:

$$v(t) = a(1 - e^{-t}) + \frac{g\tau_{in}k_0\Delta^*}{\tau_R}\frac{1}{1 - e^{-\Delta^*/\tau_{in}}}\left(e^{-t} - e^{-\frac{t}{\tau_{in}}}\right). \tag{17}$$

Now we need to verify under which conditions on $g$, in the weak and strong coupling regimes, the solution of $v(t^*) = 1$ remains close to $t^* = \Delta^*_W$ and to $t^* = \Delta^*_S$, respectively.

### B. Weak coupling

For small $g$, we have that the periodicity $\Delta^*_W$ and the evolution time are much larger than $\tau_{in}$, therefore Eq. (17) can be written as:

$$v(t) \simeq a(1 - e^{-t}) + \frac{g\tau_{in}k_0\Delta^*_W}{\tau_R}e^{-t}. \tag{18}$$

Solving $v(t^*) = 1$ we get

$$t^* \simeq \ln\left(\frac{a - g\tau_{in}k_0\Delta^*_W/\tau_R}{a-1}\right) \tag{19}$$

and then $t^* \cong \Delta^*_W = \ln(a/(a-1))$ only if $\frac{g\tau_{in}k_0\Delta^*}{\tau_R} \ll 1$, i.e. the periodicity of the weak coupling regime is preserved if $g \ll g_c^{weak}$ with:

$$g_c^{weak} = \frac{\tau_R}{\tau_{in}k_0\ln(\frac{a}{a-1})}. \tag{20}$$

### C. Strong coupling

In this case we have that the period $\Delta_S^*$ and the evolution time $t$ are much smaller than $T \simeq O(1)$. Therefore, we can approximate Eq. (17), so that:

$$v(t) \simeq at + \frac{1 - e^{-\frac{t}{\tau_{in}}}}{1 - e^{-\frac{\Delta_S^*}{\tau_{in}}}}. \tag{21}$$

Let us discuss Eq. (21) considering the two opposite regimes $\Delta_S^* \ll \tau_{in}$ and $\Delta_S^* \gg \tau_{in}$. For $\Delta_S^* \ll \tau_{in}$ also $t \ll \tau_{in}$ and we can expand Eq. (21) obtaining:

$$v(t) \simeq at + \frac{t}{\Delta_S^*} \tag{22}$$

and since $\Delta_S^* \ll \tau_{in} \ll a^{-1}$, the solution of $v(t^*) = 1$ is $t^* \simeq \Delta_S^*$. In the opposite limit, i.e. $\Delta_S^* \gg \tau_{in}$, we have $e^{-\Delta_S^*/\tau_{in}} \simeq 0$ and Eq. (21) can be approximated as:

$$v(t) \simeq at + 1 - e^{-\frac{t}{\tau_{in}}}. \tag{23}$$

Now $v(t^*) = 1$ implies that $at^* \simeq e^{-\frac{t^*}{\tau_{in}}}$ so that the firing time is of the same order of magnitude of $\tau_{in}$; this means that $t^* \simeq \tau_{in} \ll \Delta_S^*$. Therefore, in the full dynamics we obtain a self consistent solution $t^* \simeq \Delta_S^*$ which can be considered a perturbation of the strong coupling periodic evolution only for the case $\Delta_S^* \ll \tau_{in}$, i.e. only if $g \gg g_c^{strong}$ with

$$g_c^{strong} = \frac{\tau_R}{k_0 \tau_{in}^2}. \tag{24}$$

### D. Chaos in the Mean Field model

According to the above discussion, in the MF TUM model we have, for small enough $\tau_{in}$, $g_c^{weak} \ll g_c^{strong}$. We therefore expect three different regimes: for small and large values of $g$ a slow and a fast periodic dynamic should be respectively present, while in an intermediate wide range of the synaptic couplings $g_c^{weak} \ll g \ll g_c^{strong}$ the competition of the two mechanisms could give rise to a complex dynamics. We show in Fig. 2, for the MF model, the bifurcation diagrams of the temporal difference $\Delta_n \equiv t_{n+1} - t_n$ between two consecutive spikes of the network as a function of $g$ for different values of $\tau_{in}$, and the analogous values of the *coefficient of variation*, defined by the standard deviation of the interspike interval $\Delta_n$ over its mean: $\frac{\sigma_{\Delta_n}}{\langle \Delta_n \rangle}$.

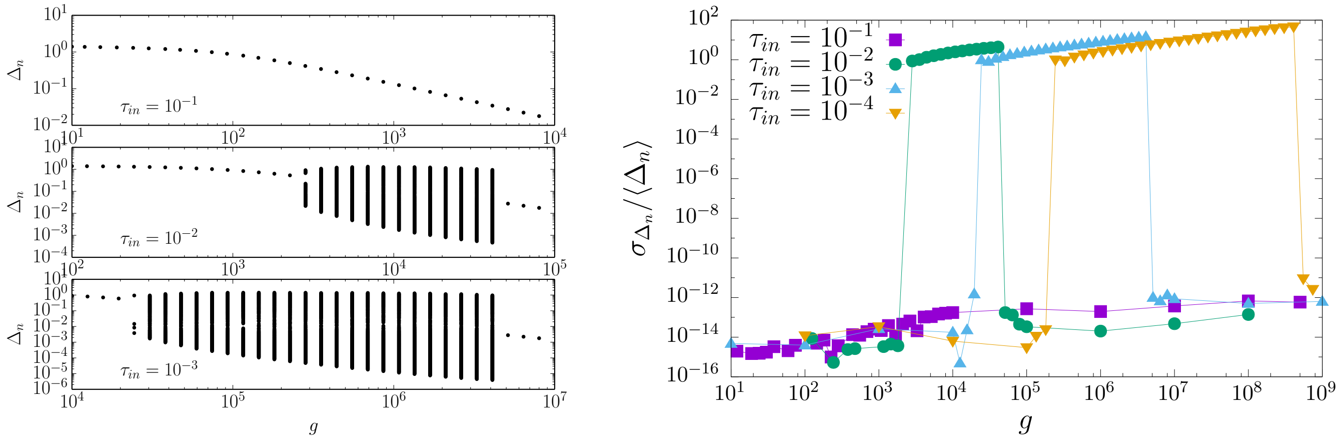


FIG. 2. Left: Feigenbaum bifurcation diagram for the MF TUM model with $\tau_{in} \neq 0$. The attractor for the interspike interval $\Delta_n$ is showed as a function of the bifurcation parameter, i.e. the coupling constant $g$. The bifurcation diagram is shown for decreasing values of the synaptic time scale $\tau_{in}$ from the top panel to the lower ($\tau_{in} = 10^{-1,-2,-3}$ respectively) in order to show the appearance and growth of the chaotic regime in the parameter space (notice that the x-axis range is different for each panel). Right: coefficient of variation of the interspike interval, $\frac{\sigma_{\Delta_n}}{\langle\Delta_n\rangle}$, for several values of $\tau_{in}$. This quantity is of order 1 in the chaotic regime only.

The calculation of the Lyapunov exponents (via the Gram-Schmidt scheme[6,7]) confirms the presence of the chaotic regime in the range of the parameter $g$ between the two bifurcations, as shown in Fig. 3. Analogous figures can be obtained for other values of $\tau_{in}$. When we consider a system of $N$ neurons coupled with the same constant $k = k_0$ this chaotic phase correspond to a regime of synchronous chaos[4,5], see Fig. 1 for a typical raster plot.

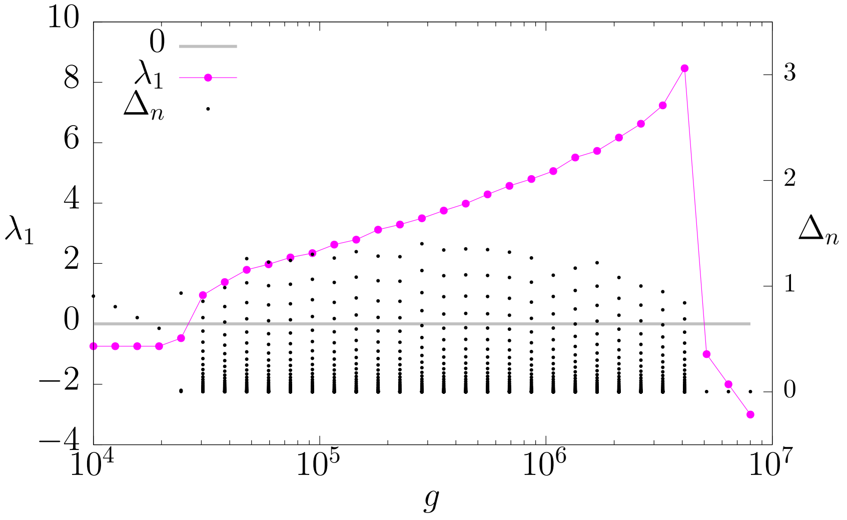


FIG. 3. First Lyapunov exponent $\lambda_1$ (in red) as a function of $g$ for the MF TUM model with $\tau_{in} = 10^{-3}$. In black, for comparison: bifurcation diagram as a function of $g$ for the same model (right x-axis). The sign of the first Lyapunov exponent $\lambda_1$ confirms a chaotic regime ($\lambda_1 > 0$) between the synchronous-bursty and bursty-asynchronous transitions outside this region ($\lambda_1 < 0$).

### E. The limit $\tau_{in} \to 0$

We now consider the MF dynamical Eq.s (5) in the limit $\tau_{in} \to 0$ and $g \to \infty$ with $g\tau_{in}$ constant, so that the new effective coupling constant is defined by $g_{\text{eff}} = k_0 g \tau_{in}$ (without loss of generality we consider $k_0 = 1$ in the rest of this section). Let us reintroduce $x = 1 - y - z$ and $x_n = 1 - y_n - z_n$ where $x_n$ are the available resources before the $n$-th firing event. If $g_{\text{eff}}(y_n + ux_n) < 1$ the evolution time $\Delta_n$ after the $n$-th firing event is larger than zero and, in particular, from the first of Eq.s (5) we obtain:

$$\Delta_n = \ln\left(\frac{a-1}{a - g_{\text{eff}}(y_n + ux_n)}\right) > 0. \tag{25}$$

Then, taking the limit $\tau_{in} \to 0$ in Eq.s (5) we get $y_{n+1} = 0$ and

$$x_{n+1} = 1 + (x_n(1-u) - 1)e^{-\Delta_n/\tau_{\text{R}}} \tag{26}$$

which is a discrete map counterpart of the differential equation:

$$\dot{x}(t) = \frac{1 - x(t)}{\tau_R} - ux(t)\sum_m \delta(t - t_{n+1}(m)). \tag{27}$$

Therefore, if $g_{\text{eff}}(y_n + ux_n) < 1$, we reduce to a single variable map for $x_n$, obtained inserting the expression (25) for $\Delta_n$ into Eq. (26).

On the other hand, if $g_{\text{eff}}(y_n + ux_n) > 1$ the solution of the first Eq. (5) can be obtained letting also $\Delta_n \to 0$ with $\frac{\Delta_n}{\tau_{\text{in}}}$ constant, so we get

$$1 = -g_{\text{eff}} \left(e^{-\Delta_n/\tau_{\text{in}}} - 1\right) (y_n + u(1 - y_n - z_n)) \tag{28}$$

or:

$$e^{-\Delta_n/\tau_{\text{in}}} = \frac{g_{\text{eff}}(y_n + ux_n) - 1}{g_{\text{eff}}(y_n + ux_n)}. \tag{29}$$

Plugging (29) into the second of (5) we have:

$$y_{n+1} = y_n + ux_n - \frac{1}{g_{\text{eff}}}. \tag{30}$$

Taking the limits $\tau_{\text{in}} \to 0$ and $\Delta_n \to 0$ in the third of (5):

$$z_{n+1} = -y_{n+1} + (z_n + y_n + u(1 - y_n - z_n)) \tag{31}$$

i.e.

$$x_{n+1} = x_n(1 - u) \tag{32}$$

as it is expected in an instantaneous firing event.

In conclusion, if $g_{\text{eff}}(y_n + ux_n) < 1$ the evolution time $\Delta_n$ is given by (25), $y_{n+1} = 0$ and $x_{n+1}$ is given by Eq. (26). If $g_{\text{eff}}(y_n + ux_n) > 1$ the evolution is instantaneous, $\Delta_n = 0$ and the maps for $x_n$ and $y_n$ are described by Eq.s (30) and (32).

An analogous limit $\tau_{in} \to 0$ can be performed also on the DMF equations obtaining for the dynamical variables $v_i(t)$ and $x_i(t)$ a set of equations similar to the TUM model described in[8]:

$$\dot{v}_i(t) = a - v_i(t) + g\tau_{in} k_i \frac{1}{N} \sum_{j=1}^{N} x_j(t) S_j(t) \tag{33}$$

$$\dot{x}_i(t) = \frac{1 - x_i(t)}{\tau_R} - ux_i(t) S_i(t) \tag{34}$$

where $g\tau_{in}$ is the new effective coupling constant. Moreover, also in this case simultaneous firing events are possible. In particular, if neuron $j$ fires at time $t_m$ and $v_i(t_m) + uN^{-1}x_j(t_m) > 1$ also neuron $i$ fires at $t_m$ and $v_i(t_m)$ is set to $v_i(t_m) + uN^{-1}x_j(t_m) - 1$. We remark that also in the DMF case, reintroducing the potential variable $v_{n+1} = g_{\text{eff}}(y_n + ux_n)$ in Eq.s (30, 32), we can eliminate $y_n$ obtaining $v_{n+1} = v_n + ug_{\text{eff}}x_n - 1$, i.e. the natural equation for a neuron that receive an input $ug_{\text{eff}}x_n$ and simultaneously fires decreasing by one unit.

In the DMF case, the dynamical description can be further summarized introducing two new indexes $m$ and $p$, labeling the firing events. The label $m$ increases of one unit each time there is a

firing event such that $\Delta_n > 0$ and $p = 1 \ldots, p_m$ labels the different simultaneous firing events. In this way we replace the index $n$ with the couple $(m, p)$: if in the firing event $\Delta_n = 0$, $m$ remains fixed and $p$ increases by one, while if $\Delta_n > 0$, $m$ increases by one and $p$ is reset to 1 ($p_m$ is the value of $p$ for which $m$ is increased to $m+1$ and $p$ is reset). With this new labels for the events, we denote $x_{(p,k)} = x_n$, $y_{(p,k)} = y_n$ and so on.

For a given value of $m$, from $p = 1$ to $p = p_m$ , Eq.s (30) and (32) can be easily evaluated obtaining:

$$x_{(m,p)} = x_{(m,1)}(1-u)^{p-1} \tag{35}$$

and

$$y_{(m,p)} = (1-(1-u)^{p-1})x_{(m,1)} - \frac{p-1}{g_{\text{eff}}} \tag{36}$$

where Eq. (36) can be verified recursively taking into account that $y_{(m,1)} = 0$. The number of simultaneous firings $p_m$ can be evaluated by verifying if $g_{\text{eff}}(y_{(p,k)} + ux_{(p,k)}) < 1$, in particular from Eq.s (35) and (36) we obtain that $p_m$ is the smallest positive integer such that:

$$gx_{(m,1)}(1-(1-u)^{p_m}) - p_m < 0. \tag{37}$$

When $p = p_m$ the time evolves of a step $\Delta_{(m,p)}$ given by (25):

$$\Delta_{(m,p_m)} = \ln\left(\frac{a-1}{a - g_{\text{eff}}(y_{(m,p_m)} + ux_{(m,p_m)})}\right) = \ln\left(\frac{a-1}{a - g_{\text{eff}}x_{(m,1)}(1-(1-u)^{p_m}) + p_m - 1}\right) \tag{38}$$

and the resources evolve according to Eq. (26):

$$x_{(m+1,1)} = 1 + (x_{(m,p_n)}(1-u) - 1)e^{-\Delta_{(m,p_m)}/\tau_{\text{R}}} = 1 + (x_{(m,1)}(1-u)^{p_m} - 1)e^{-\Delta_{(m,p_m)}/\tau_{\text{R}}}. \tag{39}$$

Finally we can plug Eq. (38) into (39) obtaining:

$$x_{(m+1,1)} = 1 + (x_{(m,1)}(1-u)^{p_m} - 1)\left(\frac{a-1}{a - g_{\text{eff}}x_{(m+1,1)}(1-(1-u)^{p_m}) + p_m - 1}\right)^{1/\tau_R} \tag{40}$$

where $p_m$ is the smallest positive integer satisfying Eq. (37). Eq. (40) represents a map for the variable $x_{(m+1,1)}$. The map (40) is shown in Fig. 4 (c.f. captions for details).

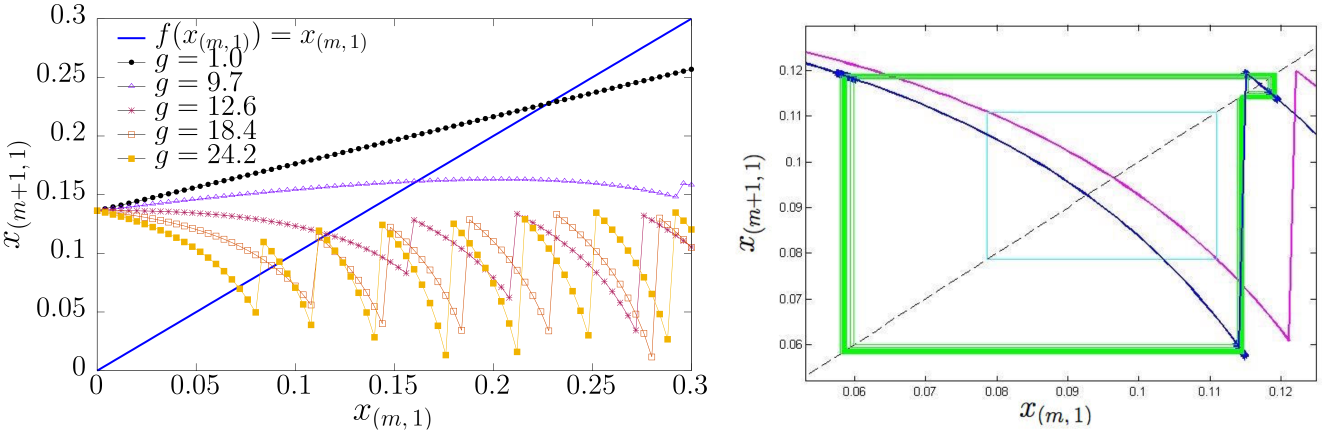


FIG. 4. Left: Map (40) for the MF TUM model with $\tau_{in} = 0$ for different values of $g_{\rm eff}$ indicated in the legend. Right: in order to highlight the difference between the quasi-synchronous and the bursty transitions, two values of $g_{\rm eff}$ are plotted in both regimes respectively. For $g_{\rm eff} = 16$ a period-two orbit is observed (light blue), while for $g_{\rm eff} = 30$ - notice that the discontinuity of the map has crossed the $y = x$ line - a chaotic behavior is present (green).

For small values of $g_{\rm eff}$ the map exhibits a stable fixed point. Increasing $g_{\rm eff}$, a stable period-two orbit is observed (see the second panel of Fig. 4). Finally, at larger values of the coupling, typically when the map features two intersections with the bisector $x_{(m+1,1)} = x_{(m,1)}$, the dynamical attractor explores a region of the phase space that cannot be confined in a limit cycle, as confirmed by the calculation of the invariant measure that presents a broad distribution (see Fig. 5). This region is strictly chaotic as the Lyapunov exponent of the map is larger then zero, as soon as the limit cycle loses stability. We remark that for $\tau_{in} \to 0$ the periodic regime at large values of $g$ does not exist. Indeed, the coupling constant $g$, for $\tau_{in} \to 0$, diverges as $g_{\rm eff}/\tau_{in}$, while the transition point between the bursty and the asynchronous regimes diverges in the same limit as $s \sim g_c^{strong} \sim \tau_{in}^{-2}$.

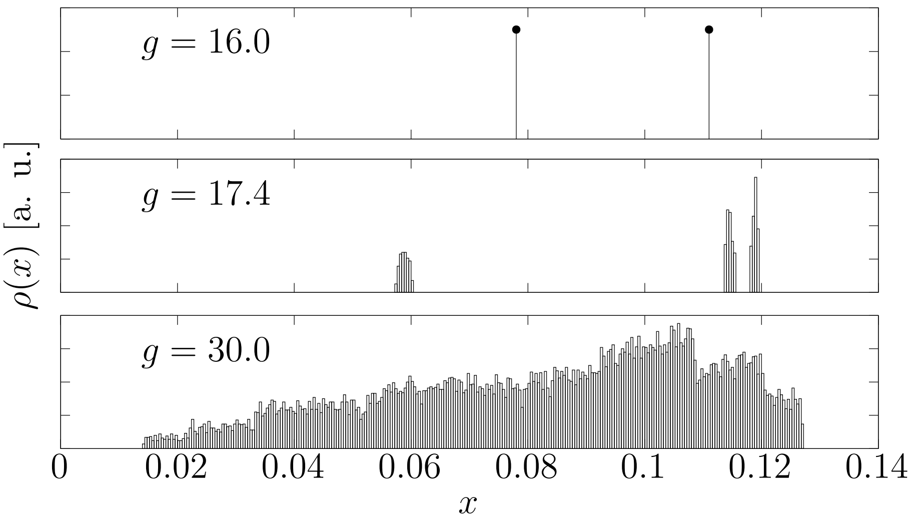


FIG. 5. Probability density $\rho(x)$ of the synaptic resource $x_n$, for $g_{\text{eff}} = 16$ (upper panel), $g_{\text{eff}} = 17.4$ (middle panel) and $g_{\text{eff}} = 30$ (lower panel). While two peaks are present for $g_{\text{eff}} = 16$, indicating a period-two orbit, a broad distribution, indicating chaotic dynamics, is observed in the last two cases.

## III. DEGREE BASED MEAN FIELD

In this section we discuss in more detail the numerical analysis of the DMF model. The DMF model consists in $N$ nodes representing neurons with coupling $gk_i$ extracted from a probability distribution $P(k_i)$. When not specified differently, the presented numerical results correspond to simulations performed with a Gaussian probability distribution $P(k_i)$, with mean $\mu = 0.7$ and variance $\sigma = 0.077$.

### A. Event driven dynamics simulation protocol

We have simulated finite size realizations of the event driven dynamics Eq.s (2), with number of neurons $N$. The temporal averages and second moments of the relevant observables (Kuramoto parameter and neuron-averaged interspike interval) are, in principle, a time integral. They have been approximated by a sum evaluated in equispaced times. E.g. $\langle f \rangle = M^{-1} \sum_{m=1}^{M} f(t, m\tau + t_0)$, where $t_0$ is a reference initial time and $\tau$ the time spacing. The parameter $\tau$ has been chosen much smaller than the average interspike, and $M$ sufficiently large, so that the results of the averages remain unchanged for larger values of $M$ and for lower values of $\tau$. We have discarded the initial *transient* regime, whose length $t_0$ is strongly dependent on the initial conditions and on the values

of the parameters. To shorten the length of the transient in series of simulations at different but close values of $g$, we take as an initial condition for the dynamic variables of a simulation at a given $g$, the final configuration attained by the simulation at the immediately lower value $g$. We have also checked the opposite protocol, reducing the value of $g$ and taking as initial condition the final configuration of the precedent simulation, verifying that both protocols lead to identical results. The stationarity of the averages and standard deviations of the Kuramoto parameter and of the interspike interval has been verified comparing the results obtained averaging over temporal windows of exponentially larger and larger width. Moreover, the width $W = \tau M$ of the temporal window is considered to be large enough if the averages of the considered observable over sub-windows of the interval (of size $b \ll W$) result statistically uncorrelated (i.e., if not only their average but their fluctuations over different sub-windows do no longer grow significantly with increasing $b$). With this method (the jackknife method), we ensure that $W$ is much larger than the correlation time of the considered observable. When we need to distinguish the time average with respect other kind of averages e.g. the average over the different neurons we use the notation $\langle \cdot \rangle_t = \langle \cdot \rangle$

### B. Global Synaptic field

Fig. 6 shows the average global synaptic field received by the neurons $g\langle Y \rangle$. It is an increasing function of $g$. As we expect from our arguments in Sec. II A, the transition between quasi-periodic/bursty and bursty/asynchronous regimes occur when $g\langle Y \rangle$ is of the same order of magnitude of the leakage term $a - v(t) \sim O(1)$. In particular, the value of $g\langle Y \rangle$ remains of order $a - v(t)$ (as shown in the first panel in Fig. 6) even for large values of $g$ (e.g. $g \sim 10^5$ in the bursty phase), since the resources are typically inactive during the evolution and $\langle Y \rangle$ assumes moderate values (notice that the amount of synaptic current received by the neurons in a given time interval scales as $g\tau_{in}$). The second panel in Fig. 6 shows that the temporal fluctuations of $gY(t)$ are larger in the bursty regime.

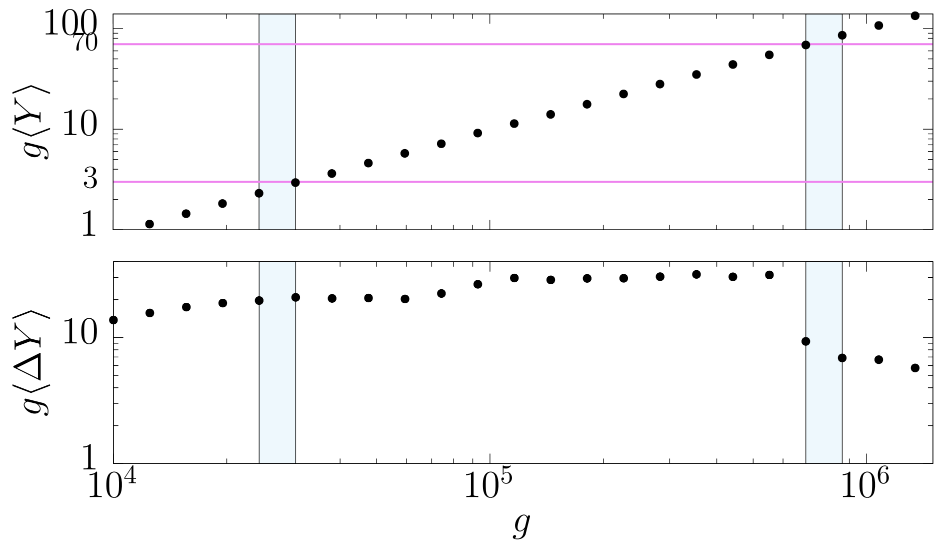


FIG. 6. Higher panel: Average global synaptic field $\langle Y\rangle$ as a function of $g$ in the Gaussian TUM model with $\tau_{in} = 10^{-3}$ and $N = 10^4$. The vertical stripes indicate the quasi-synchronous/bursty and bursty/asynchronous transitions. The horizontal line indicate the free neuron term $a - v$, revealing the value of $g$ at which the bursty regime takes place. Lower panel: fluctuations of the synaptic field, $\sigma_Y$ times $g$.

### C. Fluctuations of the interspike interval, Kuramoto parameter and global field

Let us call $\Delta_i(t)$ the interspike interval corresponding to the last two events of the $i$-th neuron, before the time $t$. The temporal average over the time index $t$, performed as described in Subsec. III A, will be denoted by $\langle\cdot\rangle_t$, while the average over the $i$ index will be denoted by $[\cdot]_i \equiv (1/N)\sum_{i=1}^{N}(\cdot)$. In the MF case, the amount of temporal fluctuations of the unique interspike $\Delta_n$ around its average is called coefficient of variation, and it is used as an order parameter discriminating among different regimes (see Fig. 2). In the more complicated case of the disordered topology, two kinds of fluctuations of the interspike interval can be defined: those with respect to $t$, averaged over $i$, and those with respect to $i$, averaged over $t$:

$$\sigma_\Delta^2 = \langle[\Delta_i^2(t)]_i - [\Delta_i(t)]_i^2\rangle_t \tag{41}$$

$$\sigma'^2_\Delta = \left[\langle\Delta_i^2(t)\rangle_t - \langle\Delta_i(t)\rangle_t^2\right]_i \tag{42}$$

While the average interspike interval is $I = \langle[\Delta_i(t)]_i\rangle_t = [\langle\Delta_i(t)\rangle_t]_i$. We observe (see Fig. 7)

that for both definitions the fluctuations present an apparent discontinuity at $g$ values compatible with the transition values (vertical stripes), at least for sufficiently large values of $N$, for which $\sigma_\Delta$ and $\sigma'_\Delta$ do no longer depend on $N$ within their error-bars. While in the asynchronous and quasi-synchronous regimes $\sigma_\Delta/I < \sigma'{}_\Delta/I$, the situation is opposite in the bursty regime, where $\sigma_\Delta/I > \sigma'{}_\Delta/I$.

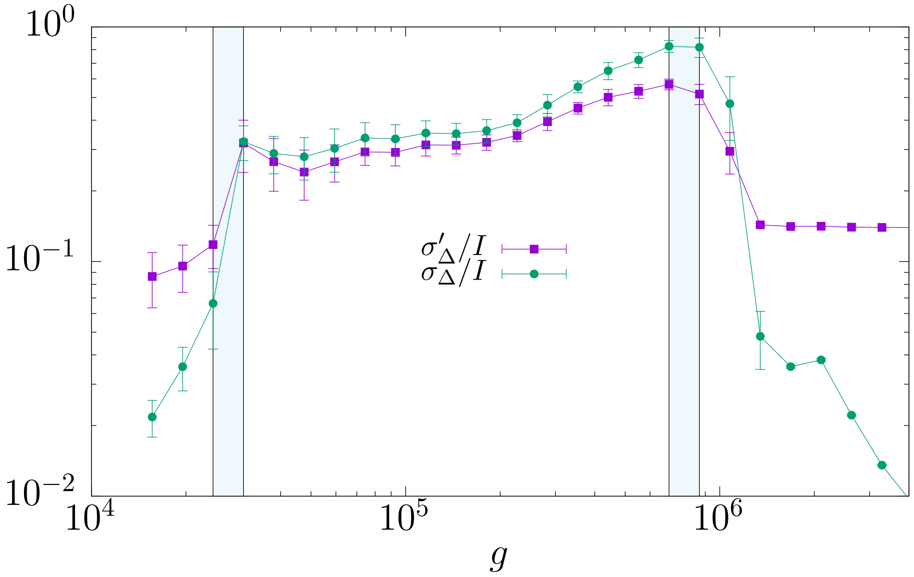


FIG. 7. Two types of fluctuations of the interspike interval $\sigma_\Delta$ and $\sigma'{}_\Delta$ as a function of $g$, for the DMF model with $N = 500$, $\tau_{in} = 10^{-3}$. The apparent discontinuity of $\sigma_\Delta$ and $\sigma'{}_\Delta$ does not coincide with the bursty-asynchronous transition: this turns out to be, however, a finite size effect absent for larger values of $N$.

Further insight about the nature of the bursty regime is provided by the Kuramoto parameter $R$ and the global field $Y$ as a function of time. Fig. 8 reveals that these quantities exhibit large temporal fluctuations.

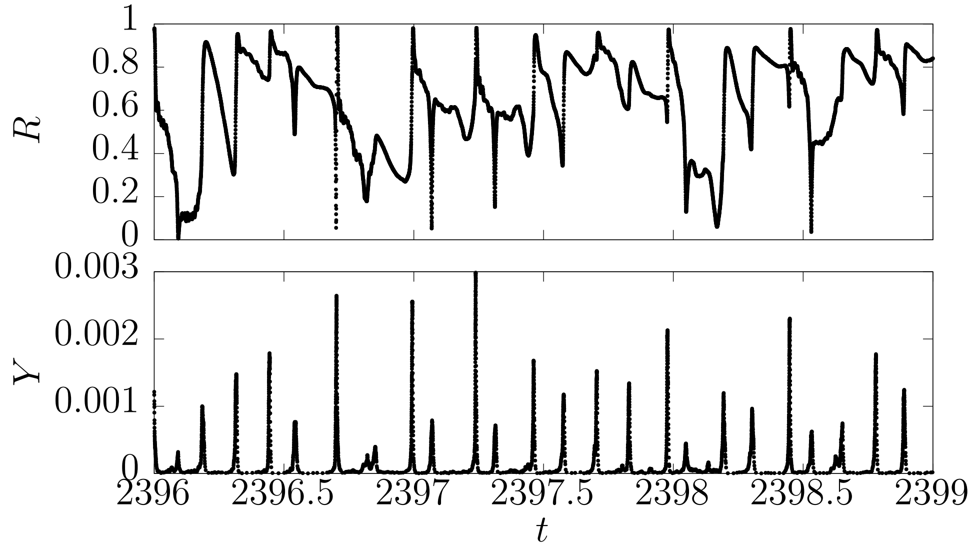


FIG. 8. Kuramoto parameter $R(t)$ (upper panel) and synaptic global field $Y(t)$ (lower panel) as functions of time in the chaotic regime ($g = 10^5,\ \tau_{in} = 10^{-3},\ N = 10^4$) in the DMF model.

### D. Lyapunov exponents

The chaotic nature of the bursty dynamical regime is then confirmed by the values of the Lyapunov exponents. Evidence is provided by numerical simulations, showing that the largest Lyapunov exponent remains positive (only) in the bursty phase, even for the largest of the simulated sizes ($N = 2 \cdot 10^4$ for $\tau_{in} = 10^{-3}$), as shown in Fig. 9 for a particular value of $g$.

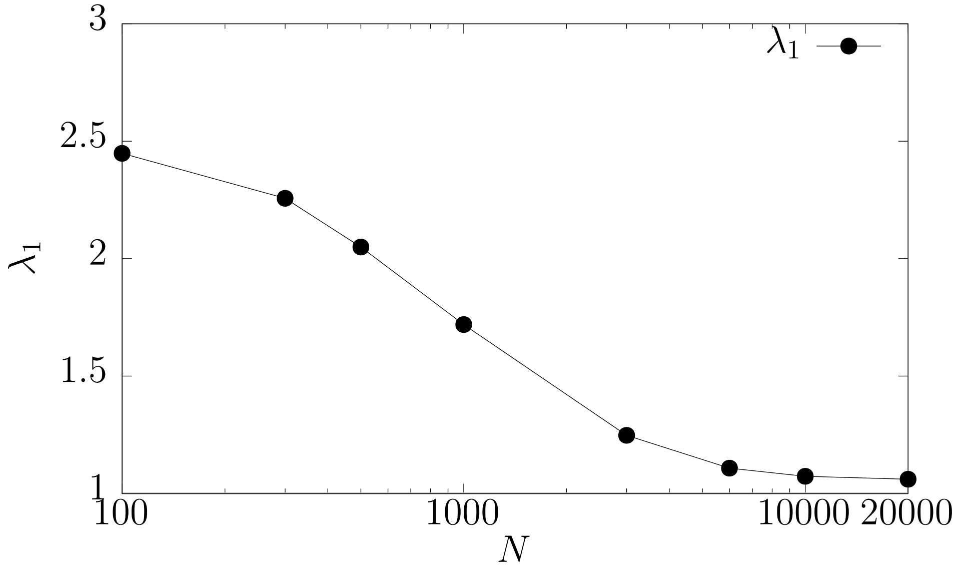


FIG. 9. Finite size scaling of the first Lyapunov exponent $\lambda_1$ as a function of the number $N$ of neurons in the DMF approach, with $\tau_{in} = 10^{-3}$ and $g = 3 \cdot 10^4$.

### E. Comparison between the DMF and MF models phase diagrams

In the DMF model with a non zero variance distribution $P(k_i)$, the two dynamical transitions occurring at $g = g_1$ and $g = g_2$, between quasi-synchronous/bursty and bursty/asynchronous behaviors, do not coincide exactly with the two corresponding transitions to chaos $g'$ and $g''$ in the pure MF model. However, in the limit of variance $\sigma \to 0$, we expect to recover the same transitions of the MF model, as the MF model corresponds to a DMF with a delta function $P(k_i)$. As a numerical confirmation, we have performed a series of simulations of the DMF model with Gaussian $P(k_i)$, with mean $\mu = 0.7$ and several decreasing values of $\sigma$. The results, in Fig. 10, show indeed that the transition points $g_1$ and $g_2$, are compatible for small $\sigma$ with the expected values (horizontal stripes) $g'$ and $g''$ of the corresponding MF model. The transitions have been estimated by means of the discontinuity of the interspike interval fluctuations.

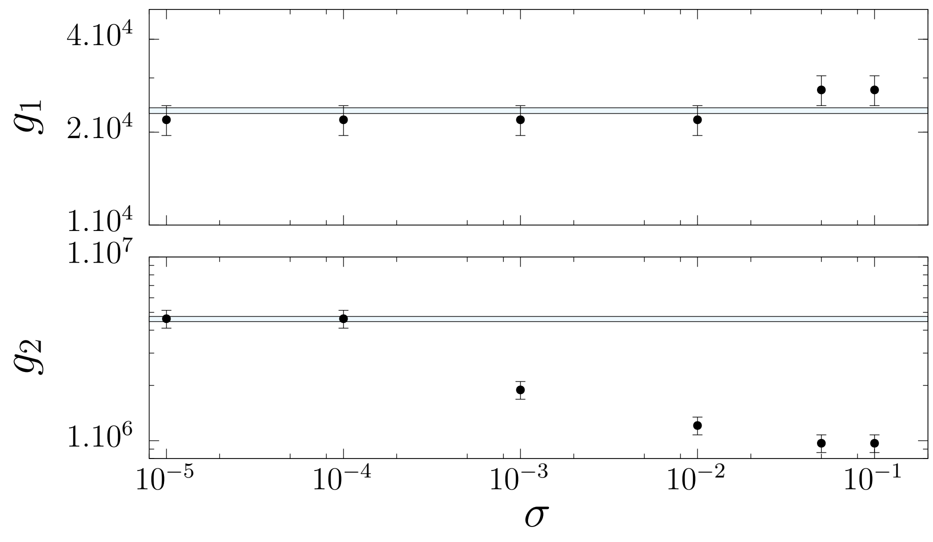


FIG. 10. Transition interval of the synaptic couplings identifying the quasi-synchronous/bursty and bursty/asynchronous transitions (upper and lower panels, $g_1$ and $g_2$ respectively) for $\tau_{in} = 10^{-3}$, as a function of the variance $\sigma$ of the Gaussian distribution $P(k_i)$, whose average is $\mu = 0.7$. The horizontal stripes indicate the two respective values of the transition to chaos, $g'$ and $g''$, in the MF model.

### F. Robustness with respect to the shape of the distribution $P(k_i)$

In the previous subsection, we verified the robustness of our results with respect to the width $\sigma$ of the Gaussian distribution, by showing that the fully MF behavior is recovered for $\sigma \to 0$. We remark that a change in the average $\mu$ of the distribution in the DMF Eq.s corresponds to a rescaling of the couplings; in particular the system with average $\mu_{\text{new}}$ displays the same dynamics of the model with average $\mu_{\text{old}}$ but with coupling $g\mu_{\text{new}}/\mu_{\text{old}}$ and variance of the distribution $\sigma\mu_{\text{new}}/\mu_{\text{old}}$. A natural question concerns the robustness of the results with respect to the shape of the coupling distribution. In Fig. 11 we plot the avalanche size distribution and the raster plot for couplings extracted from a Gamma distribution i.e.

$$P(k_i) = \gamma_{m,\theta}(k) = \frac{1}{\theta^m \Gamma(m)} k_i^{m-1} e^{-\frac{k_i}{\theta}}, \tag{43}$$

where $\Gamma(m)$ is the Euler Gamma function. Fig. 11 shows that the bursty regime is observed also in this case, in the presence of an asymmetric distribution.

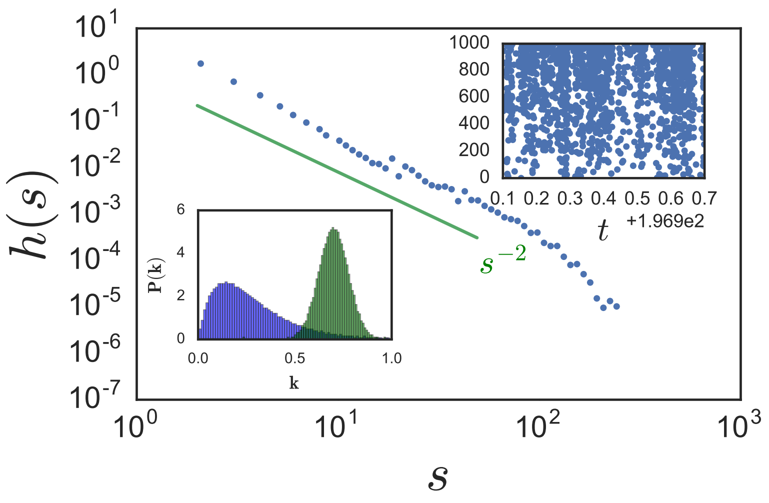


FIG. 11. Numerical results for a Gamma distribution of the couplings $P(k_i)$ defined by Eq. (43) with $m = 2$ and $\theta = 0.14$. The parameters of the simulations are $a = 1.3$, $g = 10^5$, $\tau_{in} = 10^{-3}$, $\tau_R = 10$ and the number of neurons is $N = 1000$. The main plot represents the distribution $h$ of the avalanche sizes $s$, while the upper inset is the raster plot and the lower inset is a comparison between the Gamma distribution (in blue) and the Gaussian distribution with $\mu = 0.7$ and $\sigma = 0.077$ (in green).

### G. Robustness with respect to the single neuron time scale

The phase diagram we obtained so far has been described in terms of the coupling constant $g$ and of the synaptic time scales $\tau_{in}$ and $\tau_R$. However, the system is characterized by another natural time scale, i.e. the oscillation period $T = \log(a/(a-1))$ of an isolated neuron. In our simulations $a = 1.3$ so that $T \approx 1$. Furthermore, another time scale is present in the system, the membrane time constant $\tau_m$ that rescales all time scales of the model. In practice, in order to obtain the physical value of a time scale, we need to multiply such value for $\tau_m$, and in physical system $\tau_m \approx 20 - 80$ ms.

Letting $a \to 1$ one obtains a much slower dynamics for the isolated neuron. Physically, a change in $a$ corresponds to a variation of the leakage current, which does not correspond to a trivial redefinition of the time scales since the parameter $a$ drives the non linearity of the evolution, that is the time of the resetting to zero of the potential $v_i$. In Fig. 12 we show the raster plot and the avalanches size distribution for a system with $a = 1.0001$ ($T \approx 9.2$, i.e. if $\tau_m = 30$ms we consider a neuron firing intrinsically at 3.5Hz). In this case the bursty regime is recovered for $\tau_{in} = 0.1$, so it is not necessary that $\tau_{in} \ll 1$. We remark that experimental data analysis about receptors in

the cortex suggest that the inactivation time is around 3ms (i.e. $\tau_{in} = 0.1$ if $\tau_m = 30ms$)[9,10].

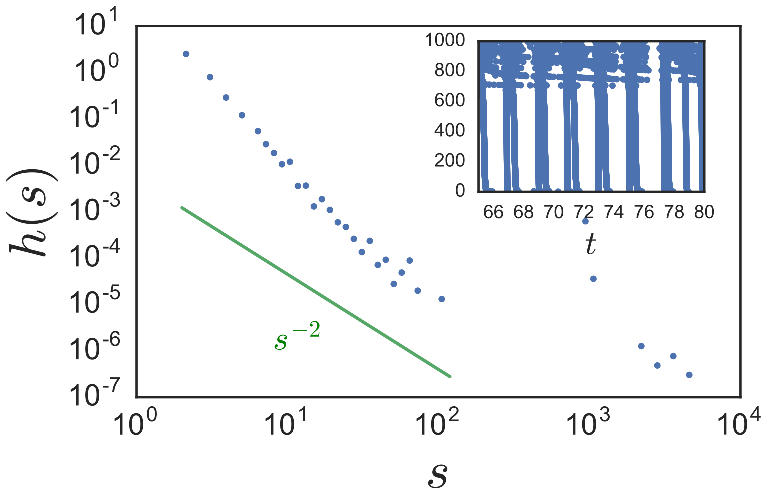


FIG. 12. Numerical results for a system with $a = 1.0001$, $g = 120$, $\tau_{in} = 10^{-1}$, $\tau_R = 10$, $N = 1000$. The coupling distribution $P(k_i)$ is a Gaussian with average $\mu = 0.7$ and variance $\sigma = 0.077$. The main plot represents the distribution $h$ of the avalanches sizes $s$, while the inset is the raster plot.

### H. Degree based Mean Field and finite connectivity systems

The results of this paper have been obtained in the framework of DMF model. In previous works[1,11] it has been shown that such an approach can be used to study also systems with large but finite connectivities; i.e. neural networks where the interactions are described by a directed adjacency matrix $A_{i,j}$ with a large enough number of incoming synapse $k_i^{in} = \sum_j A_{i,j}$. In this case the first of Eq.s (1) reads:

$$\dot{v}_i(t) = a - v_i(t) + \frac{g}{N} \sum_{j \neq i}^{N} A_{i,j} y_j(t)$$

while the last two remain unchanged.

The previous papers[1,11] refer only to the synchronous and the asynchronous regimes. In Fig. 13 we show the raster plot and the avalanches size distribution in a finite connectivity neural network in the bursty regime. In particular, we focus on a random directed network where for each node the number of incoming connections is chosen from a Gaussian distribution $P'(k_i^{in})$ with mean $N\mu$ and standard deviation $N\sigma$ and we set the parameters to a value where the DMF model exhibits burstyness. Simulations show that also in a finite connectivity networks, where a metric can be introduced, the dynamics is bursty and the avalanche distribution is characterized by a power law

whose exponent is approximatively $-2$.

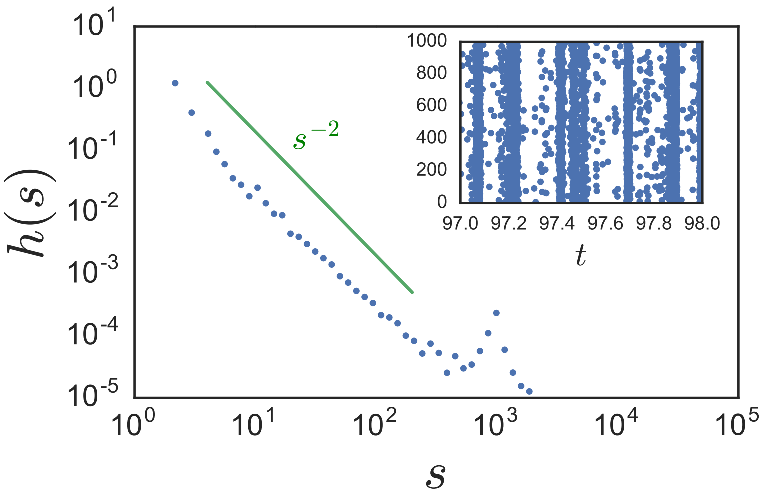


FIG. 13. Numerical results for a random finite connectivity network whit $a = 1.3$, $g = 10^5$, $\tau_{in} = 10^{-3}$, $\tau_R = 10$, $N = 1000$. The incoming degree distribution $P'(k_i^{in})$ is a Gaussian with average $\mu = 0.7N$ and variance $\sigma = 0.077N$. The main plot represents the distribution $h$ of the avalanches sizes $s$, while the inset is the raster plot.

### I. Temporal correlations

In the main article, we have defined the *connected correlation function* of the $N$-neuron system:

$$C_N(\delta) = |\langle c_N(\delta, t)\rangle_t| - |\langle c_N(T, t)\rangle_t|, \tag{44}$$

$$c_N(\delta, t) = (1/N) \sum_{n=1}^{N} e^{\imath\phi_i(t)} e^{-\imath\phi_i(t+\delta)} \tag{45}$$

where $c_N$ is the *complex correlation*, $\imath$ is the imaginary unit, and $\phi_i(t)$ is the Kuramoto phase of neuron $i$ at time $t$. The average over the time variable $\langle\cdot\rangle_t$ is performed as described in Subsec. III A.

The connected correlation, $C$, is obtained from the complex correlation by time averaging and by subtracting its asymptotic value $|\langle c_N(\mathcal{T}, t)\rangle_t|$ at a sufficiently high value of $\mathcal{T}$, such that $c_N$ does no longer significantly (beyond its fluctuations) depend on $\mathcal{T}$. At this point it is worth mentioning a delicate aspect in the numerical estimation of the asymptotic value of the correlation. In the asynchronous regime, the (disconnected) complex correlation $c_N(\delta, t)$ decreases very fast

for moderate values of $\delta$, of the order of the average interspike interval. The determination of the asymptotic correlation results therefore unambiguous. In the quasi-synchronous regime, we expect $c_N$ to achieve a non zero value for arbitrarily large values of $\delta$, at least in the large-$N$ limit, since there is a set $\mathcal{S}$ of synchronous neurons presenting a constant (and independent on time) period. In this way their Kuramoto phase delays $\phi_i(t) - \phi_i(t+\delta)$ is constant for all $\delta$ and $i \in \mathcal{S}$ and Eq. (45) remains finite for any $\delta$[11].

For finite values of $N$, however, the period of synchronized neurons is not exactly constant in time nor in the neuron index (a fact that has been related with the weak chaos exhibited by the model[1,11]). This reflects in the fact that, in the quasi-synchronous regime, $|c_N(\delta, t)|$ rapidly decays, as a function of $\delta$, and begins, as expected, to oscillate around a nonzero value which, however, begins to slowly decrease for larger values of $\delta$ (the slower the larger the value of $N$). For large $N$ and moderate $\delta$, this phenomenon is not observed in our numerical calculations, but it becomes an issue in the numerical estimation of the asymptotic value at a very large time delay $\mathcal{T}$. To construct the upper panel of Fig. 5 of the main article, we have estimated the average value of $|c_N(\mathcal{T}, t)|$, $\mathcal{T}$ being twice the maximum value of $\delta$ used in the figure abscissa, for which the asymptotic value still does not change significantly by doubling $N$ or $M$ (although, we warn, this value is not the stationary value for arbitrarily large values of $\mathcal{T}$ or $M$). In other words, to compute the quantity $C_N(t)$ in the quasi-synchronous regime, we have assumed that the quantity $c_N$ stays constant in $\delta$ for infinite $N$ (an hypothesis with which our numerical data is compatible). A similar (but less significant for the final shape of $C_N$) strong finite size effect is found in the bursty regime for large values of $\delta$. In any case, the asymptotic value reached by $|c_N(\delta, t)|$ for moderate values of $\delta$, changes abruptly with $g$: in the synchronous regime it is close, but not equal, to the squared Kuramoto parameter; for $g$ in the bursty regime, it decreases towards a number smaller than the oscillation amplitude.

We end this section proposing an alternative definition of temporal correlation function: $C'_N(\delta) = |\langle K_N(t)\, K_N(t+\delta)^* \rangle_t|$, where $K_N = (1/N) \sum_{i=1}^{N} \exp(\imath\phi_i(t))$ is the (complex) Kuramoto parameter. The qualitative behavior of both definitions is quite similar (they differ in the fact that the first definition, Eq. (44) accounts for the correlations between neurons with equal coupling $k_i$ only), although the finite size behavior of the latter definition results to be slower in our numerical analysis; we have consequently used the first definition to draw our conclusions about the temporal correlations of the system in the main article.

### J. Kolmogorov Complexity

As mentioned in the main article, we have considered the Kolmogorov complexity (KC) of the raster plot of the Gaussian model, for several values of $g$ across three model regimes. In particular, we consider the sequence of differences of spike times $\Delta_n$ (not writing the spiking neuron index), and estimate[12] the KC of such sequences as the size of the zipped file containing the sequence, divided by the size of the original file. In practical terms, we use the *gzip* algorithm to compress the file containing a sequence of $L$ spiking times (written in ascii with constant number of digits), corresponding to a simulation of the TUM model with a given set of parameters $\{\sigma\}$. We then compute $K_L$ as the ratio of the compressed file size over the original file size. We avoid writing in the original file data corresponding to the transient, by skipping a large enough amount of initial events. In this circumstance, we observe that, for large enough number of events (i.e., of lines in the original file) $L$, $K_L \simeq K$ does not depend significantly on $L$, we take then $K$ as the estimation of the KC of $\{\sigma\}$. The number of digits $n$ used to store the spiking times being large enough, has the mere influence of shifting the whole $K$ versus $\{\sigma\}$ curve by an $n$-depending constant.

In the presence of a quasi-synchronous to asynchronous regime transition, the KC presents a maximum at the parameters $\{\sigma\}$ corresponding to the transition value. This arises for a variety of types of integrate-and-fire models, as we will show in a forthcoming publication. In the presence of the bursty regime presented and characterized in this work, one observes that the bursty regime presents a higher value of the KC, the maximum of which is found for values of $g$ in the bulk bursty regime, i.e. larger than the quasi-synchronous/asynchronous transition value.

### K. Avalanche size distribution

In the main article we have presented the avalanche size distribution $h(s)$ of the DMF, exhibiting power law behavior in the bursty regime. To compute $h(s)$, the *avalanche* is defined as a set of consecutive neuronal spikes such that all the interspike intervals of such set, $\{\Delta_n\}_n$, satisfy $\Delta_n < \delta_\mathrm{t}$, where $\delta_\mathrm{t}$ is a threshold. The avalanche size distribution is consequently taken among various avalanche events during the temporal evolution. We have numerically checked that, for the cases of interest, there is a wide range of the threshold $\delta_\mathrm{t}$ (of at least two orders of magnitude), for which the avalanche size distribution does not depend significantly on it (see the left panel of Fig. 14).

With this definition, the distribution of avalanche sizes, $h(s)$, becomes broadly distributed,

as shown in Fig. 3 of the main article, and it is compatible with a power law behavior for a wide range of values of $g$ in the bursty phase ($[5.10^4 : 10^6]$, for $\tau_{in} = 10^{-3}$ and $N = 10^4, 6.10^3$), in a range of the size $s$ of roughly three orders of magnitude (see Fig. 14, right panel). The exponent $\gamma$, obtained by means of a linear fit in logarithmic scale, results to assume the values $\gamma_1 = -2.39 \pm 0.07$, $\gamma_2 = -2.07 \pm 0.04$ and $\gamma_3 = -2.08 \pm 0.05$, $\gamma_4 = -2.1 \pm 0.3$ for $g_1 \simeq 1.160 \cdot 10^5$, $g_2 \simeq 2.263 \cdot 10^5$, $g_3 \simeq 4.417 \cdot 10^5$, $g_4 = 1.07 \cdot 10^6$, respectively, for $N = 10^4$, and: $\gamma_1 = -2.42 \pm 0.25$, $\gamma_2 = -2.07 \pm 0.06$ and $\gamma_3 = -2.04 \pm 0.05$ for $N = 3 \cdot 10^3$ and the same values of $g$. The error intervals are calculated as the interval of $\gamma$ values for which the fit (performed in the intercept only) results to exhibit a value of the sum of squared residuals per degree of freedom lower than one. The fit takes into account the errors of the histogram points $h(s_i)$ (shown as error bars in the figure), which in their turn are calculated with a jackknife error estimation procedure: one blocks the data in blocks of sufficiently large size $b$, and estimates the error of $h(s_i)$ as three times the standard deviation among the different histogram points in different blocks, $\{h_j(s_i)\}_j$.

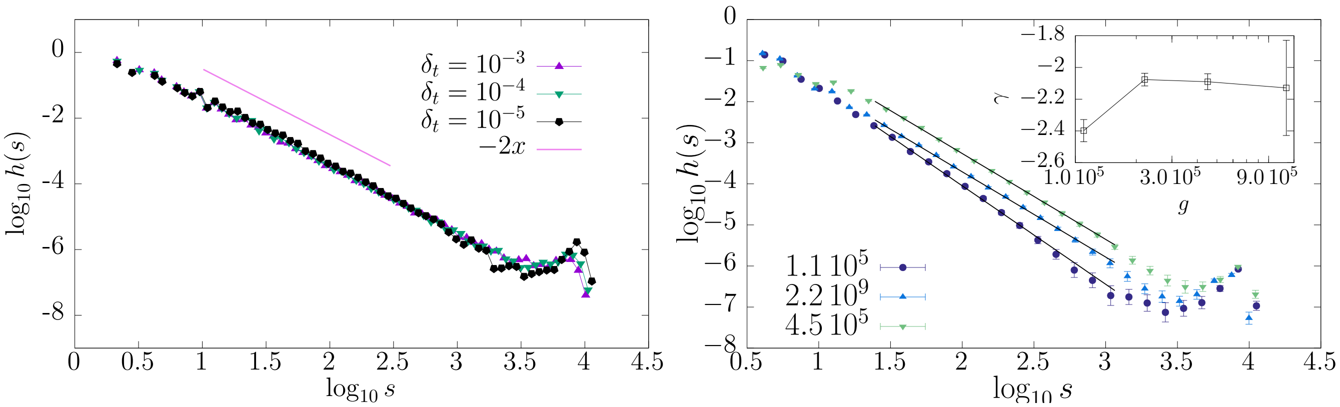


FIG. 14. Left panel: avalanche size distribution of the DMF model with $\tau_{in} = 10^{-5}$, $N = 10^4$, $g = 10^7$, for three values of the threshold $\delta_t$. Right panel: Avalanche size distribution for the system with $\tau_{in} = 10^{-3}$, $N = 10^4$ versus $g$. The straight lines are linear fits in an interval indicated by the x-axis range of the lines (the interval used for $g_4 \simeq 1.07 \cdot 10^6$ being $[2 : 3.5]$). The inset shows the value $\gamma$ of the resulting slope versus $g$, for $N = 10^4$.

---

* alessandro.vezzani@fis.unipr.it

[1] R. Burioni, M. Casartelli, M. di Volo, R. Livi, and A. Vezzani, Sci. Rep. **4**, 4336 (2014).

[2] R. Brette, Neural Comput. **19**, 2604 (2007) .

[3] M. di Volo, R. Livi, S. Luccioli, A. Politi, and A. Torcini, Phys. Rev. E **87**, 032801 (2013).

[4] M. Ding, and W. Yang, Phys.Rev. E **56**, 4009 (1997).

[5] J.F. Heagy, T.L. Carol, and L.M. Pecora, Phys.Rev. E **50**, 1874 (1994).

[6] G. Benettin, L. Galgani, A. Giorgilli, and J. M. Strelcyn, Meccanica **15**, 9 (1980).

[7] I. Shimada, and T. Nagashima, Progr. Theor. Phys. **61**, 1605 (1979).

[8] A. Levina, J. M. Herrmann, and T. Geisel, Nat. Phys. **3**, 857 (2007).

[9] M. Tsodyks, and H. Markram, PNAS **94**, 719-23 (1997).

[10] M. Tsodyks, K. Pawelzick, and H. Markram, Neural Comput. **15**, 821-35 (1998).

[11] M. di Volo, R. Burioni, M. Casartelli, R. Livi, and A. Vezzani, Phys. Rev. E **90**, 022811 (2014) .

[12] A. Kaitchenko, in *Canadian Conference on Electrical and Computer Engineering,* (IEEE, **4**, pg. 2255 2004).
